# Supplementary material for: Tuning the lattice thermal conductivity in Bismuth Telluride through Cr-doping
Source: arXiv:2008.09446 source file (2020-08-21)
Supplement: Supplementary file 1 [file Z-supp.pdf]

# Supplementary Information

## Effect of spin-lattice coupling on the lattice thermal conductivity in Cr-doped bismuth telluride

Ajit Jena, Seung-Cheol Lee,* and Satadeep Bhattacharjee†

*Indo-Korea Science and Technology Center, Bangalore*

*e-mail addresses: * seungcheol.lee@ikst.res.in, † s.bhattacharjee@ikst.res.in*

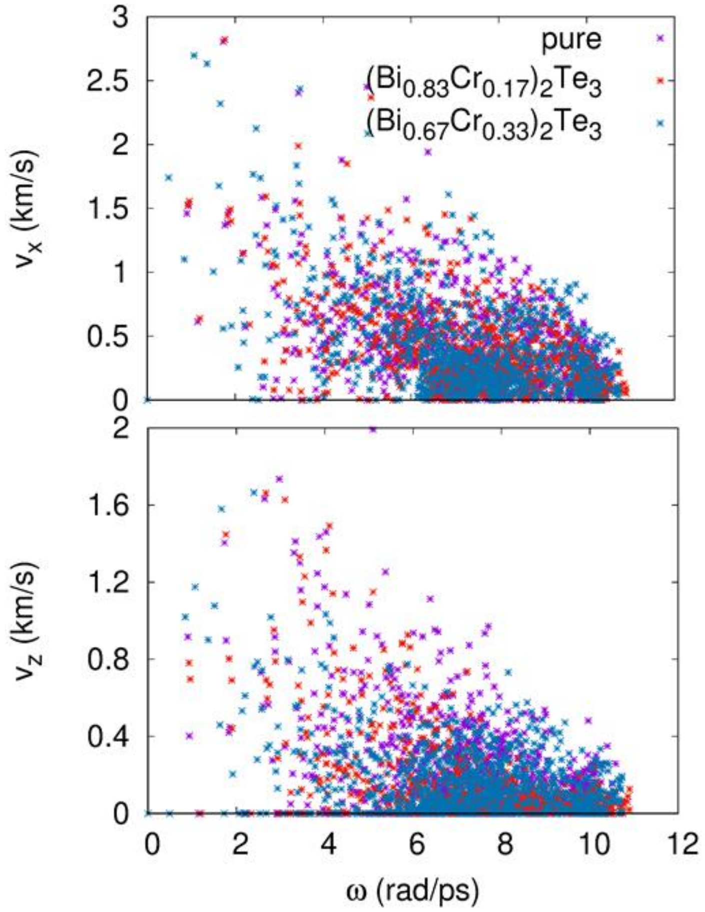


FIG. 1. Acoustic phonon group velocities of pure and Cr-doped bismuth telluride, varies with phonon frequency, along the in-plane (top) and out-of-plane (bottom) directions. In-plane component has larger value compared to the out-of-plane one. Also, it can be seen that the velocity for pure and doped cases are nearly same for each component. So, the only thing which can influence the κ is phonon anharmonicity which is discussed in detail in the manuscript.

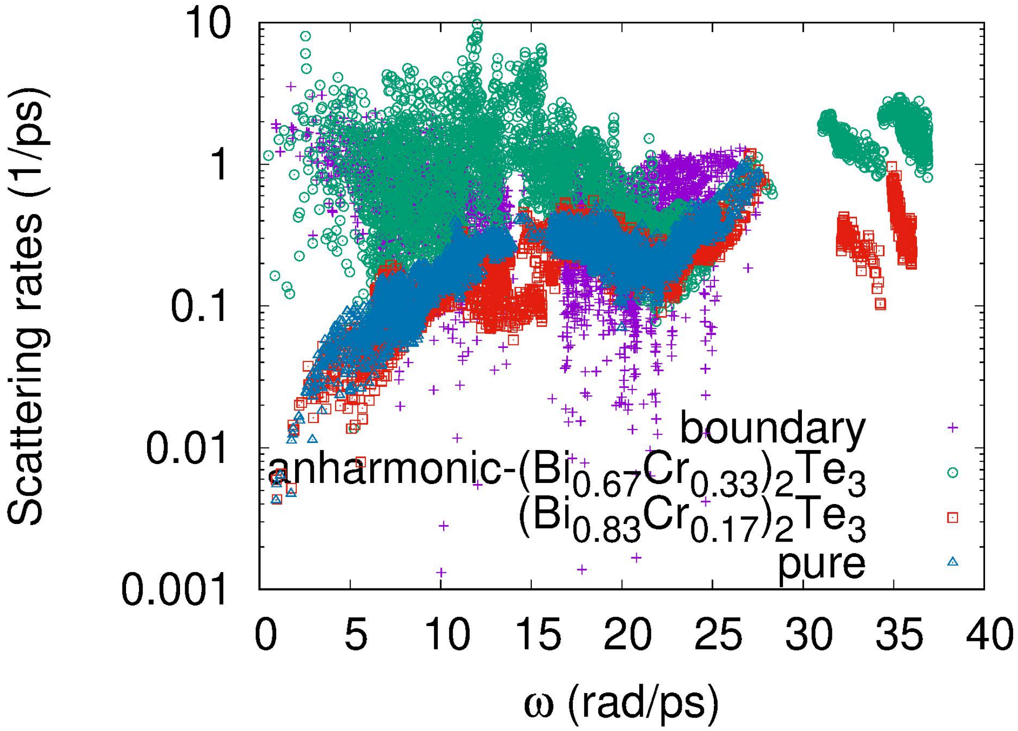


FIG. 2. Room temperature phonon-phonon (p-p) an-harmonic scattering rates of pure and Cr-doped bismuth telluride, varies with phonon frequency, compared with the boundary scattering rates. As it can be seen that the p-p scattering rates in $(Bi_{0.67}Cr_{0.33})_2Te_3$ exceeds the strong boundary scattering. Large p-p an-harmonic scattering leads to substantial reduction of the lattice thermal conductivity.
